# Supplementary material for: Thompson Sampling for Adversarial Bit Prediction
Source: arXiv:1906.09059 source file (2019-12-28)
Supplement: Supplementary file 1 [file Appendix-Dist.tex]

\section{Beta and Binomial facts}
The following is a well known property of the CDF of the $\beta(a,b)$
distribution.
\begin{fact}
\label{fact:RBF_properties} \cite[Eq.~8.17]{NIST:DLMF} For every $x
\in \left[ 0,1 \right]$ and $a,b \in \mathbb{R}$ s.t. $a,b>0$, the
following holds
\[
F_{\beta(a,b)}(x)=F_{\beta(a+1,b)}+\frac{x^{a}(1-x)^{b}}{a\mathrm{B}
\left(a,b \right)}\qquad\mbox{ and }\qquad
F_{\beta(a,b)}(x)=F_{\beta(a,b+1)}(x)-\frac{x^{a}(1-x)^{b}}{b\mathrm{B}
\left(a,b \right)}
\]
where $B(a,b)$ is the Beta function.
\end{fact}

We use the following well known approximation of the Binomials
coefficient using Stirling's approximation. (see for example, \cite{binomial})

\begin{fact}
\label{fact:das}
For every $m \in \mathbb{N}^+$ and $n \le m$ we have
\[
\binom{m}{n} = (1+o(1))\sqrt{\frac{m}{2\pi n (m-n)}} \left(\frac{m}{n}\right)^n \left(\frac{m}{m-n}\right)^{m-n} .
\]
\end{fact}

From the fact above we conclude the following lemma. (The proof is in the appendix.)

\begin{restatable}{lemma}{binombound}
\label{lem:binom-bound}
For every constant $p\in(0,1)$ and $n \ge \frac{2p}{1-p}$ ,  we have
\begin{align*}
\Pr_{X\sim Bin(\floor*{\frac{n}{p}},p)} ( X=n )= O \left(\frac{1}{\sqrt{(1-p) n}} \right).
\end{align*}
\end{restatable}
